# Supplementary material for: A Sampling-based Framework for Hypothesis Testing on Large Attributed Graphs
Source: arXiv:2403.13286 source file (2025-02-26)
Supplement: Supplementary file 1 [file appendix.tex]

\section{Appendix}\label{sec:appendix}

\subsection{Hypothesis-Agnostic Graph Samplers}
\label{app:existing_sampling_method}
Existing hypothesis-agnostic samplers fall into three categories: node, edge, and random walk based samplers. We provide details of state-of-the-art sampling methods in each category in Table ~\ref{tab:existing}.

\subsection{Convergence of Node and Edge Hypothesis Estimators}\label{app:convergence}

In this section, we construct the hypothesis estimators for node and edge hypotheses and prove their convergence for $\text{PHASE}_{\text{opt}}$. 

%%%%%%%%%%%% Node Hypothesis %%%%%%%%%%%%%%%%%
For a node hypothesis: $\textit{avg}(t_i[attr_j]|M_{t_i})$, its primary subject is $t_i[attr_j]$. Let $\mathcal{V}^* \subseteq \mathcal{V}$ be all relevant nodes satisfying $M_{t_i}$ in $\mathcal{G}$. The mean value of the node hypothesis, $\theta_{node}$, is 
\begin{equation}
 \theta_{node} = \frac{1}{|\mathcal{V}^*|}\sum_{\forall (u,v) \in \mathcal{E}} \frac{S(v)}{deg(v)}
 \label{eq:1}
\end{equation}
where $S(v) = \phi(v)[attr_j] \times \mathbbm{1}_{M_{t_i}\subseteq \mathcal{L}_{\phi(v)}}$. We assume that each edge in $\mathcal{E_S}$ is represented as $(u_i,v_i)$. Replacing $\mathcal{E}$ with $\mathcal{E_S}$, the estimator for $\theta_{node}$ is
\begin{equation}
\hat{\theta}_{node} = \frac{1}{|\mathcal{E_S} \cap \mathcal{V}^*|}\sum_{i=1}^{\mathcal{E_S}} \frac{S(v_i)}{deg(v_i)}
\label{eq:2}
\end{equation}
When $B$ goes to infinity, $\mathcal{E_S}$ converges to $\mathcal{E}$. Hence, by Theorem~\ref{thm:SLLN}, we have 
\begin{equation}
\lim_{B\to\infty} \frac{1}{| \mathcal{E_S}\cap \mathcal{V}^*|}\sum_{i=1}^{\mathcal{E_S}} \frac{S(v_i)}{deg(v_i)} \to \frac{1}{|\mathcal{V}^*|}\sum_{\forall (u,v) \in \mathcal{E}} \frac{S(v)}{deg(v)}
\label{eq:3}
\end{equation}
almost surely. Therefore, $\hat{\theta}_{node}$ is an asymptotically unbiased estimator of $\theta_{node}$.

%%%%%%%%%%%% Edge Hypothesis %%%%%%%%%%%%%%%%%
For an edge hypothesis: $\textit{avg}(r_i[attr_j]|M_{u},M_{v})$, its primary subject is $r_i[attr_j]$. Let $\mathcal{E}^* \subseteq \mathcal{E}$ be all relevant edges $(u,v)\in \mathcal{E}^*$ such that $u$ satisfies $M_{u}$ and $v$ satisfies $M_v$ respectively. The mean value of the edge hypothesis, $\theta_{edge}$, is 
\begin{equation}
 \theta_{edge} = \frac{1}{|\mathcal{E}^*|}\sum_{\forall (u,v) \in \mathcal{E}} T(v)
 \label{eq:4}
\end{equation}
where $T(u,v) = \psi(u,v)[a_j] \times \mathbbm{1}_{M_{u}\subseteq \mathcal{L}_{\phi(u)} \wedge M_{v} \subseteq \mathcal{L}_{\phi(v)}}$. Replacing $\mathcal{E}$ with a sequence of sampled edges $\mathcal{E_S}$, the estimator for $\theta_{edge}$ is
\begin{equation}
\hat{\theta}_{edge} = \frac{1}{|\mathcal{E_S} \cap \mathcal{E}^*|}\sum_{i=1}^{\mathcal{E_S}} T(u_i,v_i)
\label{eq:5}
\end{equation}
By Theorem~\ref{thm:SLLN}, we have 
\begin{equation}
\lim_{B\to\infty} \frac{1}{|\mathcal{E_S} \cap \mathcal{E}^*|}\sum_{i=1}^{\mathcal{E_S}} T(u_i,v_i) \to \frac{1}{|\mathcal{E}^*|}\sum_{\forall (u,v) \in \mathcal{E}} T(u,v)
\label{eq:6}
\end{equation}
almost surely. Therefore, $\hat{\theta}_{edge}$ is an asymptotically unbiased estimator of $\theta_{edge}$.

\subsection{Examples of Hypotheses}\label{app:hypothesis}

\begin{table}[ht!]
\caption{Examples of Hypotheses}
\vspace{-0.2cm}
\label{tab:hypo}
\resizebox{\columnwidth}{!}{%
\fontsize{14}{16}\selectfont
\begin{tabular}{|c|m{0.9\columnwidth}|c|}
\hline
\textbf{Hypothesis Type}     & \multicolumn{1}{c|}{\textbf{Example}}                                                                            & \textbf{Relevant nodes, edges, paths} \\ \hline
\multicolumn{3}{|c|}{\textbf{MovieLens}} \\ \hline
\multirow{5}{*}{Node} & \textbf{MV-N1:} The avg age of female users $>$  20                                      & 1709 (18\%)                  \\ \cline{2-3} 
                      & \textbf{MV-N2:} The avg   age of users with other occupations $>$ 20                      & 711 (7\%)                    \\ \cline{2-3} 
                      & \textbf{MV-N3:} The avg   age of male self-employed users $>$ 20                          & 190 (2\%)                    \\ \hline
\multirow{4}{*}{Edge} & \textbf{MV-E1:} The avg rating of adventure   movies $>$ 3                                & 133555 (13\%)                \\ \cline{2-3} 
                      & \textbf{MV-E2:} The avg rating of movies by artist $>$ 3                                & 49889 (5\%)                  \\ \cline{2-3} 
                      & \textbf{MV-E3:} The avg rating of musical movies by writers $>$ 3                       & 2713 (0.27\%)                \\ \hline
\multirow{7}{*}{Path} & \textbf{MV-P1:} The avg age of users who rate   both comedy and thriller movies $>$ 25    & 24157084                     \\ \cline{2-3} 
                      & \textbf{MV-P2:} The avg   age of users who have rated both documentary and sci-fi movies $>$ 25 & 375147                       \\ \cline{2-3} 
                      & \textbf{MV-P3:} The avg   age of users who have rated both documentary and crime movies $>$ 25  & 258735                       \\ \hline

\multicolumn{3}{|c|}{\textbf{DBLP}} \\ \hline

\multirow{5}{*}{Node} & \textbf{DB-N1:} The avg citation of papers published as journals $>$ 20                                                            & 199205 (13\%)               \\ \cline{2-3} 
                      & \textbf{DB-N2:} The avg   citation of papers in conferences in 2010 $>$ 10                            & 31566 (2\%)                  \\ \cline{2-3} 
                      & \textbf{DB-N3:} The avg   citation of papers published in Journal in 2017 $>$ 10                                & 1588 (0.1\%)                 \\ \hline
\multirow{5}{*}{Edge} & \textbf{DB-E1:} The avg weight of conference   papers on data mining $>$ 0.5                                    & 44925 (0.4\%)                \\ \cline{2-3} 
                      & \textbf{DB-E2:} The avg   weight of journal papers on data mining $>$ 0.5                                       & 13400 (0.12\%)               \\ \cline{2-3} 
                      & \textbf{DB-E3:} The avg   weight of papers on telecommunications network $>$ 0.5                                & 2510 (0.02\%)                \\ \hline
\multirow{6}{*}{Path} & \textbf{DB-P1:} The avg weight of papers by China's institutes on data mining $>$ 0.5              & 17671                        \\ \cline{2-3} 
                      & \textbf{DB-P2:} The avg   citation of papers co-authored by authors in Peking and China's institutions $>$ 50 & 7065                         \\ \cline{2-3} 
                      & \textbf{DB-P3:} The avg   citation of conference papers by Microsoft Researchers $>$ 50                 & 3217                         \\ \hline
                    
\multicolumn{3}{|c|}{\textbf{Yelp}} \\ \hline
\multirow{6}{*}{Node} & \textbf{YP-N1:} The avg reviews given by users   with high popularity $>$ 200                                   & 112043 (5.3\%)               \\ \cline{2-3} 
                      & \textbf{YP-N2:} The avg   stars given by users who have low prolificacy and medium popularity $>$ 3             & 16429 (0.77\%)               \\ \cline{2-3} 
                      & \textbf{YP-N3:} The avg   number of reviews of business in Illinois $>$ 70                                      & 2144 (0.1\%)                 \\ \hline
\multirow{5}{*}{Edge} & \textbf{YP-E1:} The avg ratings of fast food $>$ 4                                                            & 224536 (3.33\%)              \\ \cline{2-3} 
                      & \textbf{YP-E2:} The avg   ratings of furniture stores $>$ 3                                                     & 33040 (0.5\%)                \\ \cline{2-3} 
                      & \textbf{YP-E3:} The avg   percentage of useful reviews given by useful writers to Illinois businesses $>$ 0.5 & 4242 (0.06\%)                \\ \hline
\multirow{7}{*}{Path} & \textbf{YP-P1:} The avg rating difference on path [business in FL - high popularity user - business in LA] $>$ 0.5   &   615174                    \\ \cline{2-3} 
                      &  \textbf{YP-P2:} The avg rating difference on path [business in LA - high popularity user - business in IL] $>$ 0.5   &  15542                 \\ \cline{2-3} 
                      &  \textbf{YP-P3:} The avg rating difference on path [business in LA - medium popularity user - business in AB] $>$ 0.5   &  1080          \\ \hline
\end{tabular}%
}
\end{table}

%%%%%%%%%%%%%%%%%%%%%%%%%%%%%%%%
\begin{table*}[!t] 
\centering
\caption{Hypothesis-Agnostic Graph Sampling Methods}
\vspace{-0.2cm}
\label{tab:existing}
\begin{tabular}{|m{0.4\textwidth}|m{0.6\textwidth}|}
\hline
{\bf Node Samplers} & {\bf Descriptions} \\
\hline
Random Node Sampler \textit{(RNS)} & It uniformly samples $B$ nodes from $\mathcal{G}$~\cite{stumpf2005subnets}. \\
\hline
Degree-Based Sampler \textit{(DBS)} & It samples $B$ nodes according to their degree centrality~\cite{DBLP:journals/corr/cs-NI-0103016}. \\
\hline
PageRank-Based Sampler \textit{(PRBS)} & It samples $B$ nodes according to their page ranks~\cite{DBLP:conf/kdd/LeskovecF06}. \\
\hline
{\bf Edge Samplers} & {\bf Descriptions} \\
\hline
Random Edge Sampler \textit{(RES)} & It uniformly samples $B$ edges to form an edge-induced sub-graph~\cite{DBLP:conf/networking/KrishnamurthyFCLCP05}. \\
\hline
{\bf Random Walk Based Samplers} & {\bf Descriptions} \\
\hline
Simple Random Walk \textit{(SRW)} & It starts with a random node in $\mathcal{G}$ and proceeds by moving to the end node of a randomly selected edge connected to the current node until $B$ edges are sampled~\cite{DBLP:conf/infocom/GjokaKBM10}. \\
\hline
Frontier Sampler \textit{(FrontierS)} & It performs $m$ dependent random walks until $B-m$ edges are sampled after the initial $m$ seed nodes ~\cite{DBLP:conf/imc/RibeiroT10}. \\
\hline
Non-Backtracking Random Walk \textit{(NBRW)} & It is a variant of \textit{SRW} that does not return to the node it just left~\cite{DBLP:conf/sigmetrics/LeeXE12}. \\
\hline
Random Walk with Restarter \textit{(RWR)} & It extends \textit{SRW} with a probability to return to the starting node~\cite{DBLP:conf/kdd/LeskovecF06}. \\
\hline
Metropolis-Hastings Random Walk \textit{(MHRW)} & It adds a probabilistic acceptance condition to \textit{SRW} when moving to a neighboring node during the random walk~\cite{DBLP:journals/ton/StutzbachRDSW09}. \\
\hline
Common Neighbor Aware Random Walk \textit{(CNARW)} & It escapes tightly-knit communities sampled by \textit{SRW} by prioritizing moving to a neighboring node with higher degree and fewer common neighbors with previously visited nodes~\cite{DBLP:conf/icde/LiWL0LXL19}. \\
\hline
Community Structure Expansion Sampler \textit{(CommunitySES)} & It explores different communities in $\mathcal{G}$ using a community expansion quality score during the random walk~\cite{DBLP:conf/www/MaiyaB10}. \\
\hline
Snow Ball Sampler \textit{(SBS)} & It starts at a seed node and progressively adds a fixed $k$ neighbors until $B$ nodes are reached~\cite{goodman1961snowball}. \\
\hline
Forest Fire Sampler \textit{(FFS)} & It is a variant of \textit{SBS} with a parameterized $k$~\cite{DBLP:conf/kdd/LeskovecF06}. \\
\hline
Shortest Path Sampler \textit{(ShortestPathS)} & It samples pairs of nodes from $\mathcal{G}$ and randomly chooses a shortest path between them until $S$ has $B$ nodes~\cite{rezvanian2015sampling}. \\
\hline
\end{tabular}
\end{table*}

\begin{figure*}[tb]
    \centering
    \begin{subfigure}[b]{0.24\linewidth}
        \centering
        \includegraphics[width=\linewidth]{vldb-template/images/movielens/movielens_2-1-1_accuracy_plot_female micro.png}
        \caption{MV-N1}
        \label{fig:ml-acc-node-1}
    \end{subfigure}
    \hfill
    \begin{subfigure}[b]{0.24\linewidth}
        \centering
        \includegraphics[width=\linewidth]{vldb-template/images/movielens/movielens_2-1-1_accuracy_plot_other micro.png}
        \caption{MV-N2}
        \label{fig:ml-acc-node-2}
    \end{subfigure}
    \hfill
    \begin{subfigure}[b]{0.24\linewidth}
        \centering
        \includegraphics[width=\linewidth]{vldb-template/images/movielens/movielens_2-1-1_accuracy_plot_male_selfemployed micro.png}
        \caption{MV-N3}
        \label{fig:ml-acc-node-3}
    \end{subfigure}
    \hfill
    \begin{subfigure}[b]{0.24\linewidth}
        \centering
        \includegraphics[width=\linewidth]{vldb-template/images/movielens/movielens_2-1-1_acc-time_plot_male_selfemployed.png}
        \vspace{-0.1in}
        \caption{MV-N3}
        \label{fig:ml-time-node-1}
    \end{subfigure}

    \begin{subfigure}[b]{0.24\linewidth}
        \centering
        \includegraphics[width=\linewidth]{vldb-template/images/movielens/movielens_1-1-1_accuracy_plot_adventure micro.png}
        \caption{MV-E1}
        \label{fig:ml-acc-edge-1}
    \end{subfigure}
    \hfill
    \begin{subfigure}[b]{0.24\linewidth}
        \centering
        \includegraphics[width=\linewidth]{vldb-template/images/movielens/movielens_1-1-1_accuracy_plot_artist micro.png}
        \caption{MV-E2}
        \label{fig:ml-acc-edge-2}
    \end{subfigure}
    \hfill
    \begin{subfigure}[b]{0.24\linewidth}
        \centering
        \includegraphics[width=\linewidth]{vldb-template/images/movielens/movielens_1-1-1_accuracy_plot_musical_writer micro.png}
        \caption{MV-E3}
        \label{fig:ml-acc-edge-3}
    \end{subfigure}
    \hfill
    \begin{subfigure}[b]{0.24\linewidth}
        \centering
        \includegraphics[width=\linewidth]{vldb-template/images/movielens/movielens_1-1-1_acc-time_plot_musical_writer.png}
        \vspace{-0.13in}
        \caption{MV-E3}
        \label{fig:ml-time-edge-1}
    \end{subfigure}

    \begin{subfigure}[b]{0.24\linewidth}
        \centering
        \includegraphics[width=\linewidth]{vldb-template/images/movielens/movielens_3-1-1_accuracy_plot_thriller_comedy micro.png}
        \caption{MV-P1}
        \label{fig:ml-acc-path-1}
    \end{subfigure}
    \hfill
    \begin{subfigure}[b]{0.24\linewidth}
        \centering
        \includegraphics[width=\linewidth]{vldb-template/images/movielens/movielens_3-1-1_accuracy_plot_sci-fi_documentary_age micro.png}
        \caption{MV-P2}
        \label{fig:ml-acc-path-2}
    \end{subfigure}
    \hfill
    \begin{subfigure}[b]{0.24\linewidth}
        \centering
        \includegraphics[width=\linewidth]{vldb-template/images/movielens/movielens_3-1-1_accuracy_plot_crime_documentary_age micro.png}
        \caption{MV-P3}
        \label{fig:ml-acc-path-3}
    \end{subfigure}
    \hfill
    \begin{subfigure}[b]{0.24\linewidth}
        \centering
        \includegraphics[width=\linewidth]{vldb-template/images/movielens/movielens_3-1-1_acc-time_plot_crime_documentary_age.png}
        \vspace{-0.1in}
        \caption{MV-P3}
        \label{fig:ml-time-path-1}
    \end{subfigure}
    \vspace{-0.13in}
    \caption{Comparison of the top five sampling methods for accuracy and time (d, h, l) efficiency across three node (a, b, c), three edge (e, f, g), and three path hypotheses (i, j, k) for the MovieLens dataset.}
    \label{fig:ml-results}
\end{figure*}

We provide three hypotheses examples for each hypothesis type and dataset, as presented in Table ~\ref{tab:hypo}. Each hypothesis example has an abbreviated name in the beginning. These hypotheses are arranged in descending order of the number of relevant nodes, edges, and paths, indicated in the third column. The percentages in parentheses in this column for node and edge hypotheses are calculated by dividing the count of relevant nodes or edges by the total number of nodes or edges in the dataset, respectively. The fewer the relevant nodes, edges, or paths, the more challenging it becomes to sample a sufficient quantity for accurate hypothesis testing.

To investigate the impact of path length on the accuracy and time performance, we conduct experiments on the following two path hypotheses with lengths three and four using the DBLP dataset. 
\begin{enumerate}
    \item The average citation of two papers, each authored by a Microsoft researcher and citing each other, is greater than 50
    \item the average citation of two conference papers, each authored by a Microsoft researcher is greater than 50
\end{enumerate}
The first involves the path (author-paper-paper-author) with $l=3$ while the second relies on the path (author-paper-venue-paper-author) with $l=4$.

%%%%%%%%%%%%%%%%%%%%%%%%%%%%%%
\subsection{Experimental Result - MovieLens}\label{app:mv}

Figure~\ref{fig:ml-results} showcases the accuracy and time performance over different sampling proportions of hypotheses for the MovieLens dataset.

In terms of accuracy performance, some samplers outperform $\text{PHASE}_{\text{opt}}$ for node and edge hypotheses, and the superiority of $\text{PHASE}_{\text{opt}}$ is marginal for path hypotheses. This can be attributed to the high graph density of the MovieLens dataset, where a subgraph obtained from selected nodes has a high probability of including relevant nodes, edges, or paths as requested in $H$. For other trends of accuracy over sampling proportion, we have similar observations as described in Section ~\ref{expx:accuracy}.

Subfigures d, h, and l of Figure ~\ref{fig:ml-results} depict the accuracy versus execution time performance. Regarding node and edge hypotheses, $\text{PHASE}_{\text{opt}}$ requires slightly more time than other existing samplers to achieve comparable accuracy. This is due to the high density of the MovieLens dataset, facilitating easier sampling of relevant nodes, edges, and paths. Conversely, for path hypotheses, $\text{PHASE}_{\text{opt}}$ achieves higher accuracy in less time compared to other methods, highlighting the effectiveness of our hypothesis-aware sampling.
